# Supplementary material for: Spectroscopy of Quantum-Dot Orbitals with In-Plane Magnetic Fields
Source: arXiv:1804.00162 ancillary file (2018-03-31)
Supplement: Supplementary file 1 [file supplementary.pdf]

# SUPPLEMENTAL MATERIAL

# Spectroscopy of Quantum-Dot Orbitals with In-Plane Magnetic Fields

Leon C. Camenzind,[1] Liuqi Yu,[1] Peter Stano,[2,3,4] Jeramy Zimmerman,[5]
Arthur C. Gossard,[5] Daniel Loss,[1,2] and Dominik M. Zumbühl[1]

[1] *Department of Physics, University of Basel, Basel 4056, Switzerland*
[2] *Center for Emergent Matter Science, RIKEN, Saitama 351-0198, Japan*
[3] *Department of Applied Physics, School of Engineering, University of Tokyo, 7-3-1 Hongo, Bunkyo-ku, Tokyo 113-8656, Japan*
[4] *Institute of Physics, Slovak Academy of Sciences, 845 11 Bratislava, Slovakia*
[5] *Materials Department, University of California, Santa Barbara 93106, USA*

(Dated: 31 / 3 / 2018)

**CONTENTS**

S1. Calculated wave functions 1

S2. Total energy correction due to in-plane magnetic field and ground-state behavior 2

S3. Calculated energies of the ground- and excited orbital states 4

S4. Shape invariance of lever arm $\alpha_P$ 5

S5. Measuring excited orbital states 7

References 9

## S1. CALCULATED WAVE FUNCTIONS

We calculate the wave functions using the solution of the three dimensional anisotropic oscillator with confinement frequencies $\omega_{x,y,z} = E_{x,y,z}/\hbar$. We do not account for the triangular confinement potential along the z-direction for which the solutions of the Schrödinger equation are Airy functions, since for $n_z = 0$, the difference of these confinements are found to be very small for the wave functions considered here[1]. Hence, we get

$$\Psi_{n_x,n_y,n_z} = \sqrt[4]{\frac{m^3\omega_x\omega_y\omega_z}{\hbar^3}} \cdot \frac{\exp\left(-\frac{m(\omega_x x^2+\omega_y y^2+\omega_z z^2)}{2\hbar}\right)\cdot}{\sqrt{2^{n_x+n_y+n_z}n_x!n_y!n_z!\pi^{3/2}}} \cdot H_{n_x}\left(\sqrt{\frac{m\omega_x}{\hbar}}x\right) H_{n_y}\left(\sqrt{\frac{m\omega_y}{\hbar}}y\right) H_{n_z}\left(\sqrt{\frac{m\omega_z}{\hbar}}z\right) \quad (1)$$

where $H_n$ is the n-th Hermite polynomial. Fig. S1-1 shows the solutions for the ground state and the first excited states along the excitation axes $x$ and $y$ for the three configurations discussed in the main text. In contrast to the exaggerated schematics in the main text, these realistic calculations only show subtle differences in real space between the configurations.

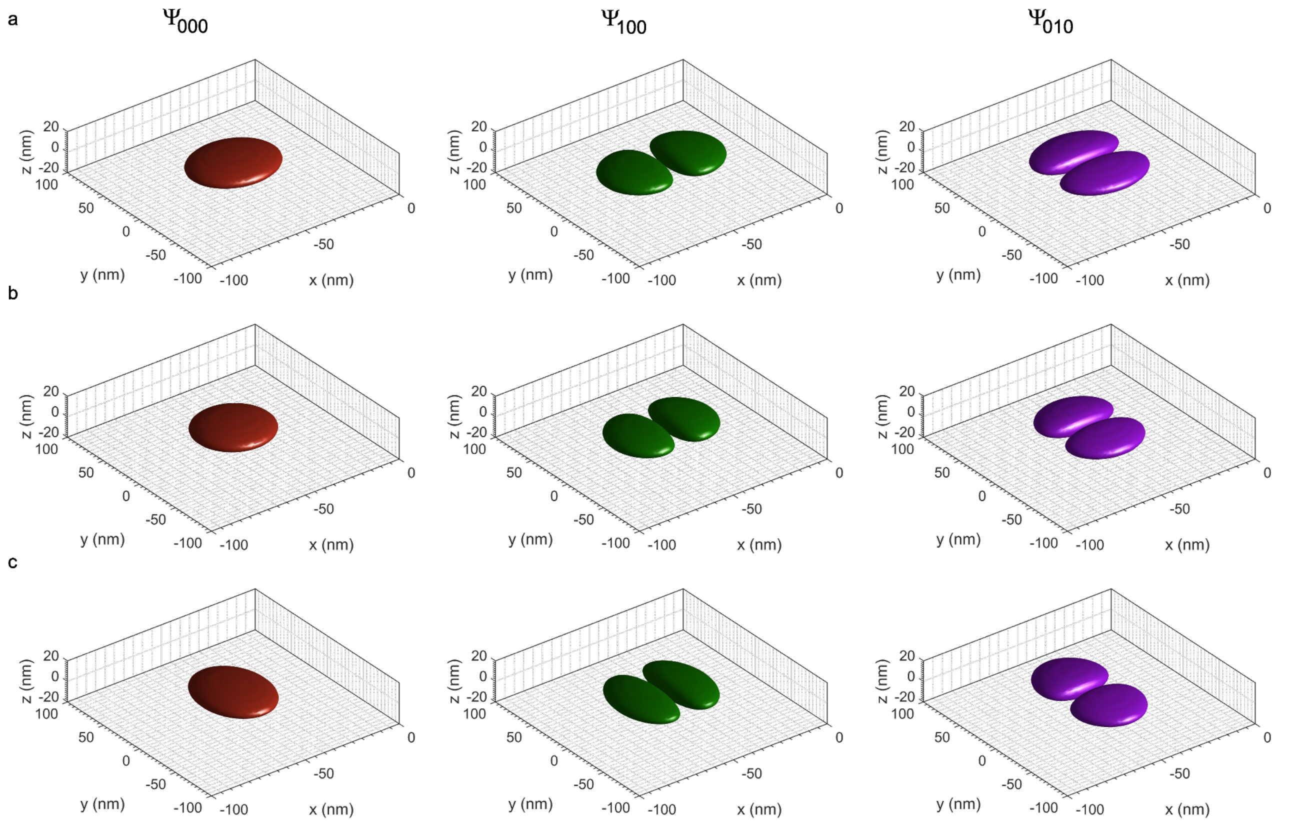


FIG. S1-1. Spatial representation of the wavefunctions $|\Psi_{n_x,n_y,n_z}|^2$ for a probability of presence larger than 90% for configurations (a) $V_{\text{shape}} = -900$ mV ($E_x = 1.8$ meV, $E_y = 2.7$ meV), (b) $V_{\text{shape}} = -550$ mV ($E_x = 2.4$ meV, $E_y = 2.6$ meV) and (c) $V_{\text{shape}} = -300$ mV ($E_x = 3$ meV, $E_y = 1.8$ meV).

## S2. TOTAL ENERGY CORRECTION DUE TO IN-PLANE MAGNETIC FIELD AND GROUND-STATE BEHAVIOR

To avoid notation confusion, we defined the orbital energies $E_{x,y}$ as the energy difference from the orbital ground state to the excited orbital states. All energies presented in the main text are defined with respect to the spin-ground state of the orbital ground state. The latter is a direct consequence of the measurement scheme which is explained in Sec. S5 in more detail. In the zero-field case, $E_{x,y}(B = 0)$ is the energy difference of the harmonic oscillator levels. When a field is applied, $E_{x,y}$ becomes a more abstract energy scale conceivable as an increase of the particle mass of the harmonic oscillator. More precisely and as described in Ref.[1], for the particle mass in the direction perpendicular to the magnetic field $m_\perp$, we obtain a mass renormalization due to a magnetic flux $\Phi = (e/\hbar)B\lambda_z^2$ given by

$$\frac{1}{m_\perp(\Phi^2 \ll 1)} \approx \frac{1}{m_\perp(\Phi = 0)}\left(1 - \Phi^2\right) \tag{2}$$

in the low field limit and

$$\frac{1}{m_\perp(\Phi^2 \gg 1)} \approx \frac{1}{m_\perp(\Phi = 0)}\left(\frac{1}{1 + \Phi^2}\right) \tag{3}$$

in the high field limit. Here $\lambda_z$ is the effective width of the wave function along the growth direction penetrated by the magnetic field $B$.

As also derivated in Ref.[1], the magnetic field-induced energy correction to the total energy of the state $(n_x, n_y)$ is

$$\delta E_{n_x,n_y} = -\frac{\Phi^2}{2}\left[\hbar\omega_x \sin^2(\delta-\phi)\,(n_x+1/2) + \hbar\omega_y \sin^2(\delta+\pi/2-\phi)\,(n_y+1/2)\right] \tag{4}$$

where $\hbar\omega_{x,y}$ are the ladder spacings of the bi-harmonic oscillator at zero field and $\delta$ defines the dot orientation (see Fig. 1). The energy $\hbar\omega_{x,y}$ corresponds to $E_{n_x,n_y}(B=0)$ in our measurements because we can only measure orbital energies relative to the ground-state energy with spectroscopy method (see Sec. S5). Therefore, the ground state dependence on the magnetic field has to be added to our data in order to obtain the energy correction of the harmonic oscillator. Note that Eq. (4) is a result for small fields ($\Phi \ll 1$) when ignoring inter-subband corrections which is justified when only the lowest sub-band of the 2DEG is occupied ($n_z = 0$). In Fig. S2-1, we show the two data sets of Fig. 3 as corrections of the total energy by including the ground state energy correction. Here it is recognized that in contrast to the spectroscopy measurements shown in Fig. 3, the effective energy modification of the orbital perpendicular to the field ($E_x + E_{GS}$) is rather small compared to the orbital oriented parallel to field ($E_y + E_{GS}$) because of increasing $E_{GS}$.

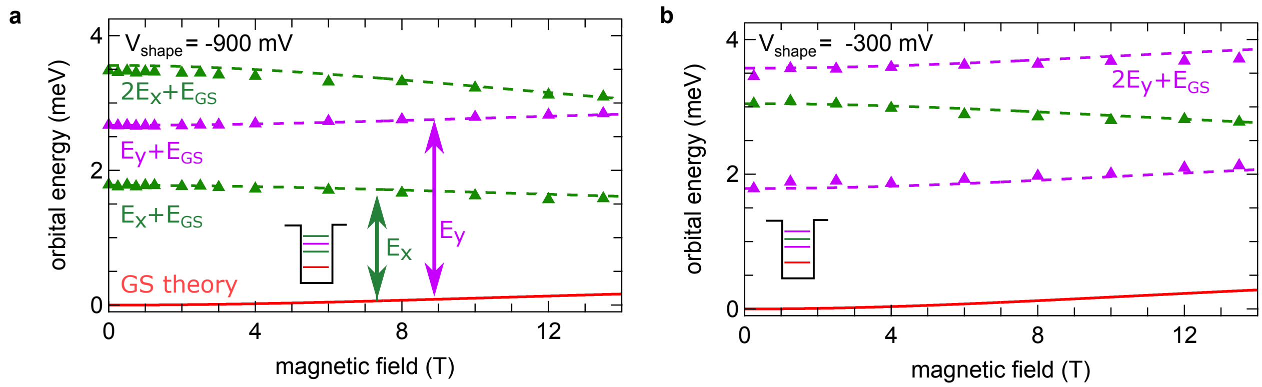


FIG. S2-1. Magnetic field-indcued energy corrections to the ground state (red) and excited orbital states (green, purple) for (a) $V_{\text{shape}} = -900\,\text{mV}$ and (b) $V_{\text{shape}} = -300\,\text{mV}$. The data for the excited states (triangles) was obtained by adding the theoretically predicted ground state shift to data of Fig. 3. $E_x$ and $E_y$ indicate the energy measured in the experiment by the excited orbital state spectroscopy technique.

## S3. CALCULATED ENERGIES OF THE GROUND- AND EXCITED ORBITAL STATES

From the experiment we are able to extract all parameters needed to calculate $E_{n_x,n_y}(B, \phi, \delta, \hbar\omega_x, \omega_y, \omega_z)$ using Eq. (4). In Fig. S3-1, we present $B-\phi$ diagrams of the induced energy corrections for the three configurations ($V_{\mathrm{shape}} = -900, -550$ and $-300\,\mathrm{mV}$) discussed in the main text. Here, we use $\delta \sim 225°$ and assume that the quantum dot is aligned with the device coordinate system. Hence the small tilt ($\delta \sim 215 \pm 1°$) which is found for $V_{\mathrm{shape}} = -550\,\mathrm{mV}$ is neglected for these calculations (see Fig. 3).

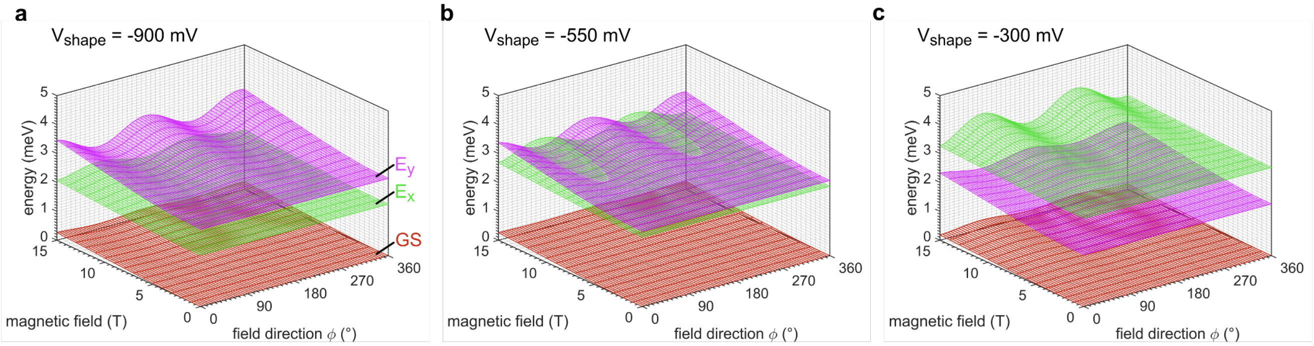


FIG. S3-1. Calculated energy dependence of the ground state (red), x-like (green) and y-like (dark purple) orbital excited state for an in-plane magnetic field with angle $\phi$ and field strength $B$ for configurations (a) $V_{\mathrm{shape}} = -900$ mV ($E_x = 1.8$ meV, $E_y = 2.7$ meV), (b) $V_{\mathrm{shape}} = -550$ mV ($E_x = 2.4$ meV, $E_y = 2.6$ meV) and (c.) $V_{\mathrm{shape}}300$ mV ($E_x = 3$ meV, $E_y = 1.8$ meV). Interestingly, for the situation in (b) a crossing of the excited orbital energies is predicted for certain magnetic field directions. The emerging of such a crossing is identified in the data in Fig. 3.

## S4. SHAPE INVARIANCE OF LEVER ARM $\alpha_P$

The lever arm for different shapes $V_{\text{shape}}$ (Fig. 2) is obtained via charge sensing thermometry by probing the Fermi-Dirac occupation distribution of the electrons in the reservoir connected to the quantum dot (see Fig. 1) at an increased temperature of $T = 300$ mK[2,3]. Therefore, we open the tunnel barrier such that the ground state shows a coupling rate of a few hundreds Hz. This coupling is still well below the bandwidth of our charge sensor ($\sim 30$ kHz measured using Low Noise/High Stability I to V converter SP983 by Basel Electronics) which allows us to measure resonant tunneling in real time when the dot ground state level is placed within the temperature broadening $k_BT$ at the chemical potential $\mu$ (Fig. S4-1(a)). Monitoring the conductance of the charge sensor $G_{sensor}$ for certain waiting time $t_w$ (about 5 s) allows us to calculate the dot occupation probability $P_{on}$ by analyzing how long the dot was filled and respectively, empty during $t_w$. To do so we have to be able to discriminate the charge state during $t_w$ (Fig. S4-1(b)). Therefore, a charge state separation threshold is determined retrospectively from $G_{sensor}$ histograms (dashed line Fig. S4-1(c)). Using this threshold the real time trace is binarized (seen as green and blue curve in Fig. S4-1(b)) The total time the dot has been occupied is $T_{on}$ and respectively, empty $T_{off}$ during $t_w$. Then $P_{on} = T_{on}/(T_{on}+T_{off})$ is calculated.

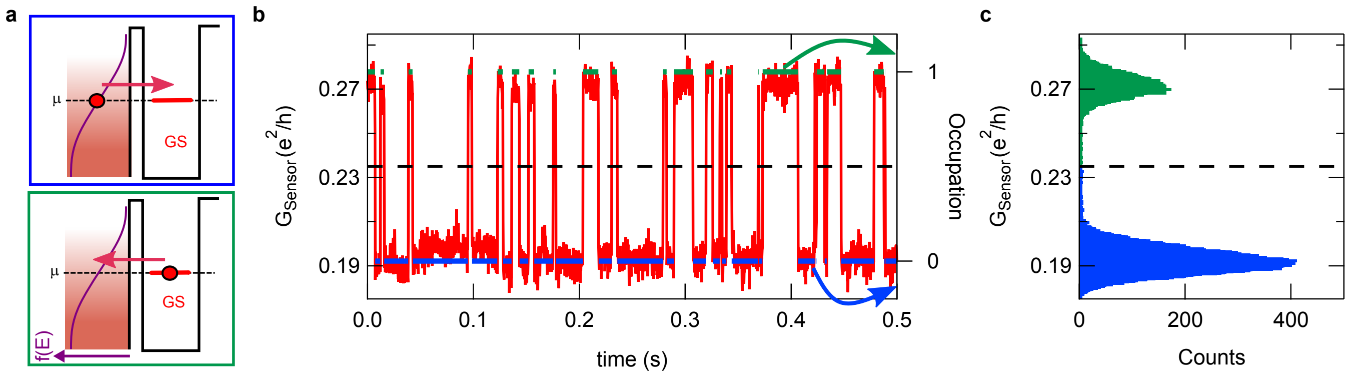


FIG. S4-1. (a) Resonant tunneling occurs when the level of the quantum dot is aligned with the Fermi-Dirac temperature broadened occupation distribution $f(E)$ around the chemical potential $\mu$ of the reservoir. At this energies, occupied as well as unoccupied states are available in the reservoir (lower panel). Therefore, electrons can tunnel from filled state into the empty quantum dot (upper panel) or from the occupied quantum dot into an empty state of the reservoir. When the tunnel barrier is tuned accordingly, this leads to electrons tunneling in and out of the dot as a function of time. (b) In the sensor $G_{sensor}$ the resonant tunneling is recognized as a fluctuating two-level system. (c) Histogram of $G_{sensor}$ allows to reliably define a charge state separation threshold with which the charge states are assigned in measurements such as shown in (b), indicated with the green (charged dot) and blue (empty dot) traces. From this, the total charging probability $P_{on}$ and also the tunnel-rate[4] are calculated.

Measuring $P_{on}$ for various detuning $\Delta V_P$ exhibits

$$P_{on}(\Delta V_P) = \left(1 + \frac{1}{2}\exp\left(\frac{-e\cdot\alpha_P\cdot(\Delta V_P - V_P)}{k_BT}\right)\right)^{-1} \tag{5}$$

with $V_P$ being a voltage offset, $\alpha_P$ the lever arm and $k_BT$ the thermal energy of the electrons in the reservoir. In general, the temperature of the electronic system is larger than the mixing chamber temperature of the dilution refrigerator ($\approx 25$ mK)[5]. Also a wider distribution is beneficial to later reduce the effective error on the extracted lever arm, we, therefore, heat up the system to 300 mK where the electronic temperature equals to the temperature of the mixing chamber. In Fig. S4-2, we show $P_{on}(\Delta V_P)$ for a dot shape configuration $V_{\text{shape}} = -900$ mV (see Fig. 2).

Because this technique is very sensitive to stochastic charge rearrangements in the semiconductor[3], we repeat this measurement between 3 and 10 times.

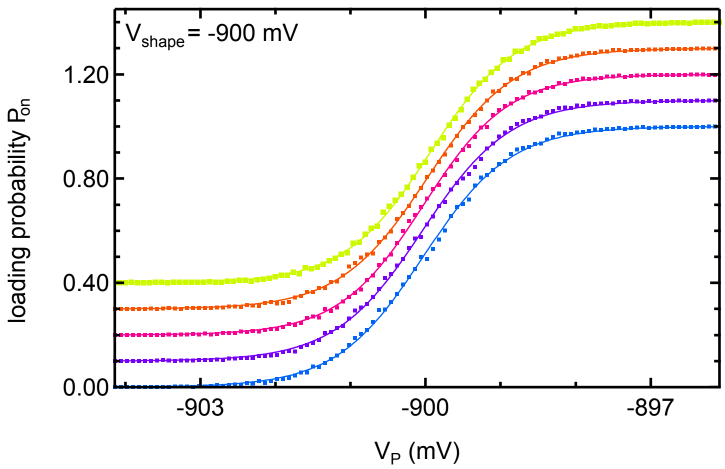


FIG. S4-2. Dependence of the quantum dot occupation probability $P_{on}$ as a function of detuning $\Delta V_P$ obtained for a shape $V_{\text{shape}} = -900\,\text{mV}$ at a temperature of 300 mK. Different traces correspond to various repetitions and are offset for clarity.

We fit each measurements individually to $P_{on} \sim 1/\left(1 + 0.5 \cdot \exp\left(-(\Delta V_p - V_P)/z\right)\right)$ where $1/z = \alpha_P/k_bT$. Fig. S4-3 presents data for the configurations of $V_{\text{shape}}$ showed in Fig. 2. The extracted fit-parameter $z$ only shows a small deviation for different repetitions which indicates that this method gives consistent and reliable results. We also show data for $V_{\text{shape}} = -200\,\text{mV}$. At this configuration, the gate voltages at the plunger gates ($V_{LP} = V_{CP} = V_{RP} = -200\,\text{mV}$) are very small and are barely enough to deplete the 2DEG underneath. This leads to a very soft confinement potential at the bottom side of the device and the quantum dot is defined closer to gate CP leading to a sharp increase in the lever arm compared to the other configurations (see also Fig. S4-4(b)). Because of the soft confinement, charges can be trapped under these gates which significantly complicates gating of the system (e.g. by pulsing). Therefore the pulsed gate spectroscopy data for this configuration is unreliable and is not presented in the text.

In Fig. S4-4 we compare $z$ as well as the resulting $\alpha_P$ for different shape configurations. We apply similar voltages to the gates LW and RW and balance these changes with LP, CP and RP which share the nominal voltage. The voltage on the nose N is found by adjusting the tunnel barrier between LW and N such that the tunnel coupling to the reservoir is in the range of 10 to 100 Hz. Since the quantum dot shape manipulation is balanced to keep the dot in the center of the device, without $V_{\text{shape}} = -200\,\text{mV}$, the lever arm $\alpha_P$ shows only a weak dependence on the shape configuration $V_{\text{shape}}$ The gate voltages for different configurations $V_{\text{shape}}$ are found to be highly reproducible even for multiple cool-downs.

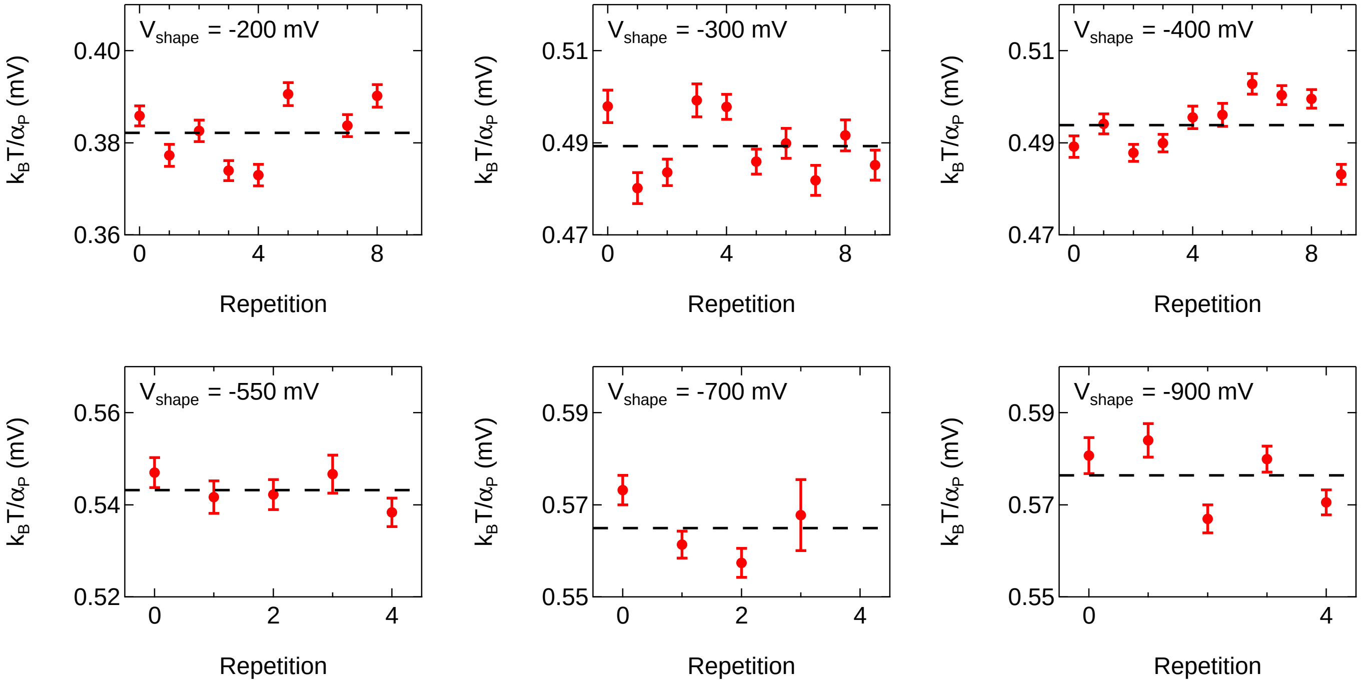


FIG. S4-3. Extracted fit parameter $z = k_b T/\alpha_P$ from measurements of the Fermi-Dirac distribution for different shape configurations.

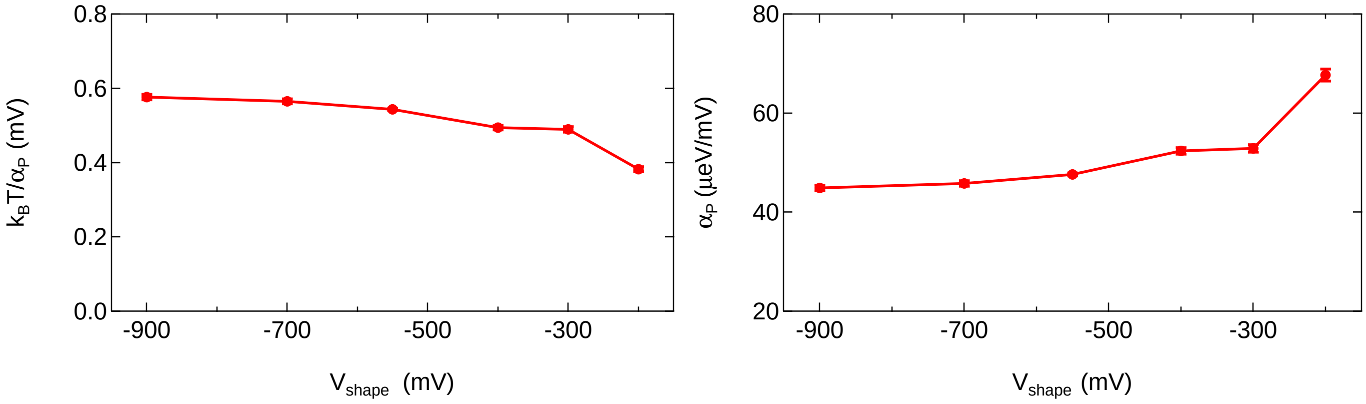


FIG. S4-4. Different $V_{\text{shape}}$ also leads to change in the capacity of the dot to plunger gate CP and therefore levararm $\alpha_P$. $\alpha_P$ is obtained by probing the Fermi-Dirac distribution of the reservoir by charge sensing thermometry at 300 mK[3].

## S5. MEASURING EXCITED ORBITAL STATES

Our spectroscopy of quantum dot orbitals strongly relies on the ability to measure the coupling of the orbital excited states to the reservoir[6]. In this section we provide some additional experimental details on how this coupling is measured.

We obtain the orbital excitation energies, by measuring the coupling of the single-particle states in an empty quantum dot to the connected reservoir. For the situation in which an excited orbital state (EOS) is in resonant with the chemical potential of the reservoir $\mu$ (see Fig. 1), it is energetically more favorable for the electrons to

tunnel into the energetically lower orbital ground state. As soon as an electron has tunneled on the dot, the dot goes into Coulomb blockade which prevents additional electron tunneling into EOS. Therefore, the the EOS has to be brought into resonance with $\mu$ on a timescale much faster than the GS is filled. Experimentally, this is achieved by pulsing the single particle energy states of the empty quantum dot faster than the tunnel rate in to the GS. In this situation electrons prefer to tunnel into the energetically higher excited state because this states couples stronger to the reservoir than the orbital ground-state[7]. There are two reasons for this increased coupling. For a rectangular barrier, the transmission coefficient $T(E) \sim exp(-2\sqrt{2m/\hbar^2 \cdot |V_0 - E|})$ as found in WKB approximation is exponentially sensitive to energy detuning with respect to the chemical potential of the reservior. Therefore, the potential through which the electrons have to tunnel is much larger for the energetically more detuned GS (see Fig. 1(b)). For the same reason,coupling of the EOS becomes exponentially suppressed once detuned from$\mu$ as indicated with the black dotted curves in Fig. 1(c). Also, the spatial span of the excited orbital states is increased compared to the ground state (see Fig. S1-1). This leads to an larger overlap of the quantum dot wave function with the wave functions of the electrons in reservoir and results in an increased tunnel coupling.

In the experiment the coupling of the first excited states is found to be orders of magnitudes stronger. The device is tuned such that the tunnel coupling of the GS is between 10-100 Hz which leads to EOS couplings of tens of kHz. We note that different coupling of the individual EOS has been observed when manipulating the shape of the quantum dot because of accompanied changes in orientation and extent of the wave function. The EOS coupling rates often exceed the bandwidth of our charge sensor ( 30 kHz) and are therefore note directly resolvable. We overcome this limitation by exploiting the fact that the pulse bandwidth of our gates (~1 MHz[4]) exceeds the sensor bandwidth by orders of magnitudes. Therefore, this fast couplings can be resolved by having the EOS resonant with $\mu$ for a pulse duration $t_w$ when applying pulses to the plunger gate CP (see Fig. S5-1(a)). An electron tunneling into an EOS will decay into the orbital ground state under the emission of a phonon[8] (Fig. 1(b)). This process happens on GHz timescale and leads to the electron being trapped in the orbital GS. After $t_w$, the dot is pulsed such that the GS is resonant with $\mu$ and the charge sensor conductance $G_{Sensor}$ is monitored for 500$\mu$s which allows to discriminate if the pulse lead to a charging of the dot. Because of the finite tunnel coupling of the GS to the reservoir, four different events are distinguishable in the read-out time: either the dot is empty or charged or an electron tunnels out respectively in to the dot. These events are detected and taken into account for the statistics of the charging probability $P_{on}$. For the tunnel rates and read out times chosen, only a few percent of the read out traces actually show a tunneling event which reduces the amount of misinterpreted read out outcomes due to missed events. To illustrate the measurement outcome, we present the dependence of $P_{on}$ on different amplitudes $\Delta V_p$ and waiting times $t_w$ in Fig. S5-2. Here, the EOS are observed as sharp increases of $P_{on}$ for different $t_w$ given by their individual coupling. The loading probability is $P_{on} = 1 - e^{-\Gamma_{in} \cdot t_w}$ which allows us to obtain $\Gamma_{in}$ by fitting to $P_{on}(t_w)$. Because the general scaling of the coupling (e.g. coupling of GS) is different, it is not useful to compare values of the coupling $\Gamma_{in}$ of particular measurements. In interest of time, we therefore often conducdt the excited orbital spectroscopy for one carefully chosen $t_w$ and only extract the energies of the EOS.

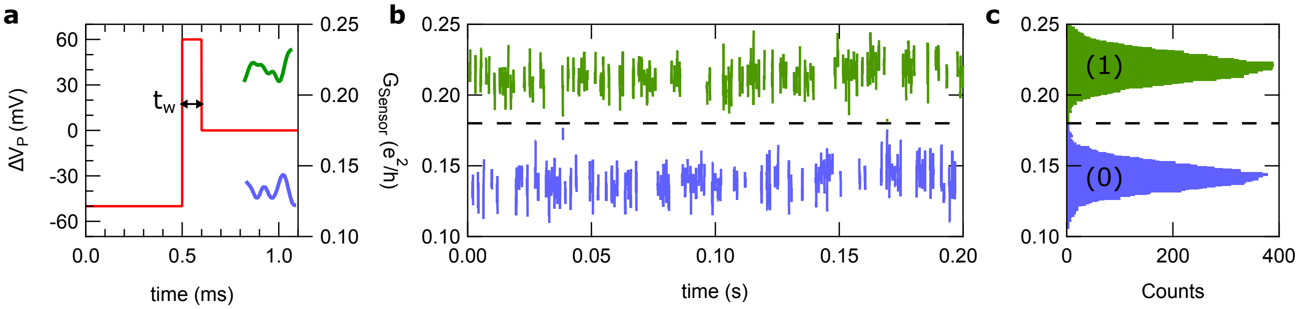


FIG. S5-1. (a) Examplary shape of a three step pulse applied to gate CP for $\Delta V_P = 60\,\mathrm{mV}$ (red trace): in the first 0.5 ms the dot is depleted at a negative energy detuning. The dot is then pulsed into the charging state for $t_w = 0.1\,\mathrm{ms}$ in this case. To read-out the dot is pulsed such that the orbital ground state is resonant with the chemical potential $\mu$. Here the charge sensor is monitored for about $200\,\mu\mathrm{s}$. Because the specific sensor conductance $G_{Sensor}$ for the charge states are known, this allows to determine if the dot is empty (blue trace) or if it has been charged during the charging step (green trace). The first $300\,\mu\mathrm{s}$ during the read-out state are cut because the sensor has to relax from the capacitive cross-talk from the large pulse amplitudes applied here. (b) An assembled segment of 180 read-out traces out of a 2000 pulse sequence used to resolve the charging probability $P_{on}$. (c) Histogram of the values of the charge sensor during read-out confirms the capability to distinguish the charge states in a single shot measurement. Here, the total counts for both charge states are very comparable which indicates $P_{on}$ 0.5.

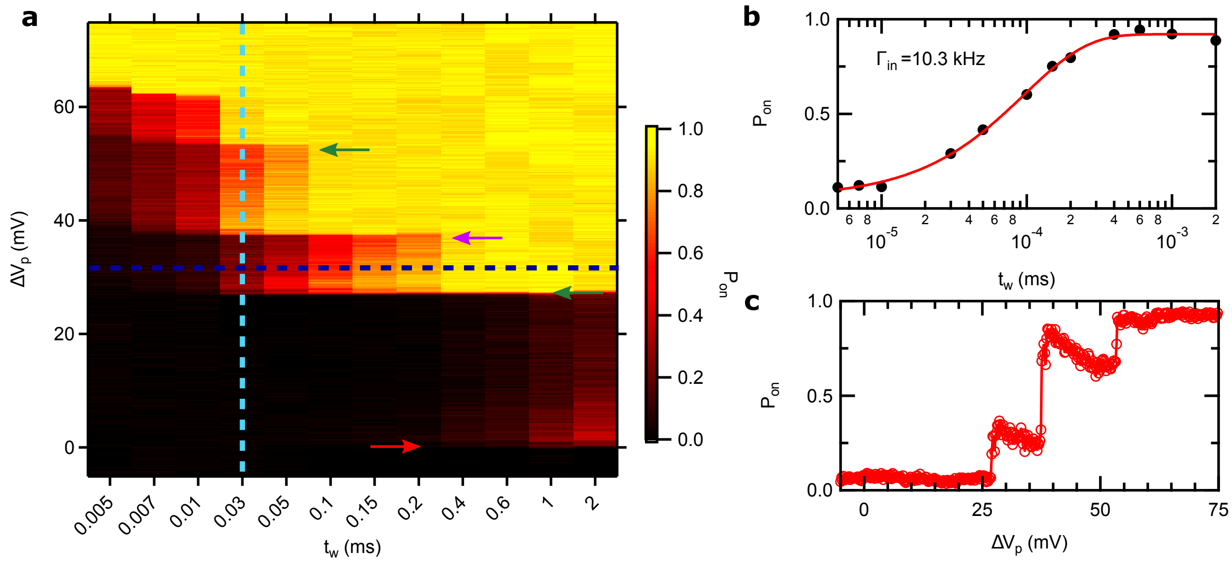


FIG. S5-2. (a) Probability for the dot being loaded after charge pulse with depth $\Delta V_p$ and waiting time $t_w$ for a configuration $V_{\text{shape}} = -700\,\mathrm{mV}$. The arrows depict the ground state (red) as well as the x-like (green) and y-like (purple) excited orbital states. Note that the x-axis is not linear. (b) Cut along $t_w$ as indicated with the bright blue line in (a). By fitting an exponential function, the total coupling of the quantum dot $\Gamma_{in}(\Delta V_P)$ is obtained. (c) Cut along the dark blue line in (a) shows all states. For most of the measurements, spectroscopy with a single $t_w$ was performed whereas $t_w$ was chosen such that all relevant states are resolved.

[1] Stano, P. *et al.* Gated 2DEG quantum dot in a strong in-plane magnetic field: orbital effects (2017). Preprint.

[2] Gustavsson, S. *et al.* Counting statistics and super-poissonian noise in a quantum dot: Time-resolved measurements of electron transport. *Phys. Rev. B* **74**, 195305 (2006). URL `https://link.aps.org/doi/10.1103/PhysRevB.74.195305`.

[3] Maradan, D. *et al.* Gaas quantum dot thermometry using direct transport and charge sensing. *J. Low Temp. Phys* **175**,

784–798 (2014). URL https://link.springer.com/article/10.1007/s10909-014-1169-6.

[4] Camenzind, L. C. *et al.* Hyperfine-phonon spin relaxation in a GaAs single electron quantum dot. *arXiv:1711.01474* (2017). URL http://arxiv.org/abs/1711.01474.

[5] Casparis, L. *et al.* Metallic Coulomb blockade thermometry down to 10 mK and below. *Rev. Sci. Instrum.* **83**, 083903 (2012). URL http://aip.scitation.org/doi/10.1063/1.4744944.

[6] Amasha, S. *et al.* Electrical control of spin relaxation in a quantum dot. *Phys. Rev. Lett.* **100**, 046803 (2008). URL https://link.aps.org/doi/10.1103/PhysRevLett.100.046803.

[7] Liles, S. D. *et al.* Spin filling and orbital structure of the first six holes in a silicon metal-oxide-semiconductor quantum dot (2018). URL http://arxiv.org/abs/1801.04494. 1801.04494.

[8] Stano, P. & Fabian, J. Control of electron spin and orbital resonances in quantum dots through spin-orbit interactions. *Phys. Rev. B* **77**, 045310 (2008). URL https://link.aps.org/doi/10.1103/PhysRevB.77.045310.
